# Supplementary material for: Projection Regret: Reducing Background Bias for Novelty Detection via Diffusion Models
Source: arXiv:2312.02615 source file (2023-12-05)
Supplement: Supplementary file 1 [file supp.tex]

\documentclass{article}

% if you need to pass options to natbib, use, e.g.:
\PassOptionsToPackage{numbers}{natbib}
% before loading neurips_2023

% ready for submission
\usepackage{neurips_2023}

% to compile a preprint version, e.g., for submission to arXiv, add add the
% [preprint] option:
%     \usepackage[preprint]{neurips_2023}

% to compile a camera-ready version, add the [final] option, e.g.:
%     \usepackage[final]{neurips_2023}

% to avoid loading the natbib package, add option nonatbib:
%    \usepackage[nonatbib]{neurips_2023}

\usepackage[utf8]{inputenc} % allow utf-8 input
\usepackage[T1]{fontenc}    % use 8-bit T1 fonts
\usepackage{hyperref}       % hyperlinks
\usepackage{url}            % simple URL typesetting
\usepackage{booktabs}       % professional-quality tables
\usepackage{amsfonts}       % blackboard math symbols
\usepackage{nicefrac}       % compact symbols for 1/2, etc.
\usepackage{microtype}      % microtypography
\usepackage[table]{xcolor}  % colors
\usepackage{bm}
\usepackage{enumitem}
\usepackage{amsmath,amsthm,amssymb}
\usepackage{mathtools}
\usepackage{multirow}
\usepackage{outlines}
\usepackage{enumitem}
\usepackage{caption}
\usepackage{subcaption}
\usepackage{algorithm}
\usepackage{listings}
\usepackage{algpseudocode}
\usepackage{arydshln}
\usepackage{wrapfig,booktabs}
\usepackage{pifont}
\makeatletter
\def\adl@drawiv#1#2#3{%
        \hskip.5\tabcolsep
        \xleaders#3{#2.5\@tempdimb #1{1}#2.5\@tempdimb}%
                #2\z@ plus1fil minus1fil\relax
        \hskip.5\tabcolsep}
\newcommand{\cdashlinelr}[1]{%
  \noalign{\vskip\aboverulesep
           \global\let\@dashdrawstore\adl@draw
           \global\let\adl@draw\adl@drawiv}
  \cdashline{#1}
  \noalign{\global\let\adl@draw\@dashdrawstore
           \vskip\belowrulesep}}
\makeatother

\usepackage{pifont}% http://ctan.org/pkg/pifont
%
%

 % thin space, limits underneath in displays

\hypersetup{colorlinks,citecolor={blue}}

\definecolor{Gray}{gray}{0.9}

\usepackage{xspace}
\newcommand{\methodname}{Projection Regret\xspace}

\title{\methodname: Reducing Background Bias \\ for Novelty Detection via Diffusion Models}

% The \author macro works with any number of authors. There are two commands
% used to separate the names and addresses of multiple authors: \And and \AND.
%
% Using \And between authors leaves it to LaTeX to determine where to break the
% lines. Using \AND forces a line break at that point. So, if LaTeX puts 3 of 4
% authors names on the first line, and the last on the second line, try using
% \AND instead of \And before the third author name.

\author{}
%\author{
%Sungik Choi \\ 
%LG AI Research
%\texttt{sungik.choi@lgresearch.ai} \\
%\And
%Hankook Lee \\
%LG AI Research
%\texttt{hankook.lee@lgresearch.ai} \\
%\And
%Moontae Lee
%\texttt{moontae.lee@lgresearch.ai}
%}

 % parameter theta ?

\begin{document}

\begin{center}
{\LARGE \bf Supplementary Material} \\
\end{center}
\vspace{-0.15in}
\begin{center}
{\Large \bf Projection Regret: Reducing Background Bias \\ for Novelty Detection via Diffusion Models}
\end{center}

\appendix
\input{appendix}

\bibliography{main}
\bibliographystyle{unsrtnat}

\end{document}
